# Supplementary material for: Deep Volumetric Ambient Occlusion
Source: arXiv:2008.08345 source file (2020-10-16)
Supplement: Supplementary file 1 [file supmat.pdf]

# Deep Volumetric Ambient Occlusion
# Supplemental Material

Dominik Engel and Timo Ropinski

July 28, 2020

## 1 Comparison with Traditional Techniques

Figure 1 shows renders of the resulting AO volume from our comparison with LAO (compare Table 3 in the paper). Note how LAO manages to get the contrast and overall brightness of the AO right with very few samples, while producing artifacts. DVAO on the other hand can vary from the ground truth in contrast and overall brightness, while producing smooth results. As we noted in Section 4.2 in the paper, the SSIM metric does not penalize those deviations as strong as MSE, which is why LAO outperforms DVAO in terms of MSE already with few samples, despite its artifacts.

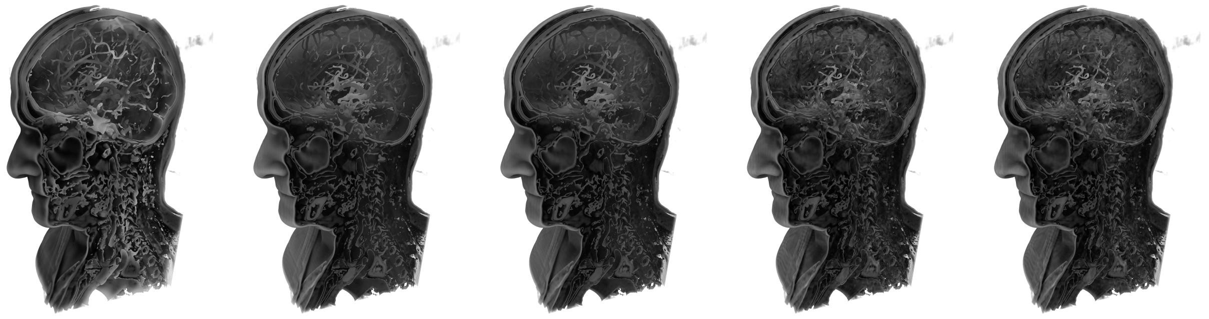

(a) DVAO (b) Ground Truth (c) LAO-190 (d) LAO-32 (e) LAO-16

Figure 1: Comparison of DVAO and LAO with different amounts of rays.

## 2 Failure Cases

Here we discuss failures of DVAO regarding visual quality. As we already stated in the main paper, DVAO tends to produce results with higher contrast compared to the ground truth and the overall brightness can deviate as well. Figure 1a shows a clear example of this effect. DVAO's prediction in this figure has significantly higher contrast and is overall brighter than the ground truth. We found that the brightness issue can be easily resolved by scaling the AO results to be brighter or darker during rendering. Since AO is used to improve depth perception locally, it is generally hard to determine our training ground truth as ”the one” correct result for AO, meaning that shifts in brightness do not necessarily impair the depth perception and it is not uncommon to adjust AO brightness during rendering anyways. The higher contrast often results in tiny structures being a lot more pronounced compared to the ground truth. Compare for example the small details inside the head of Figure 1a. In practice we actually found this behaviour rather useful, because the small structures are more easily distinguishable in the rendering compared to the ground truth AO, however this might also be misleading. Since we have trained DVAO to produce AO as defined implicitly through our training ground truth data, we would expect that this behavior does not occur. Future work should consider incorporating constraints to enforce overall brightness and contrast. This might be possible through regularization.

## 3 Training Data

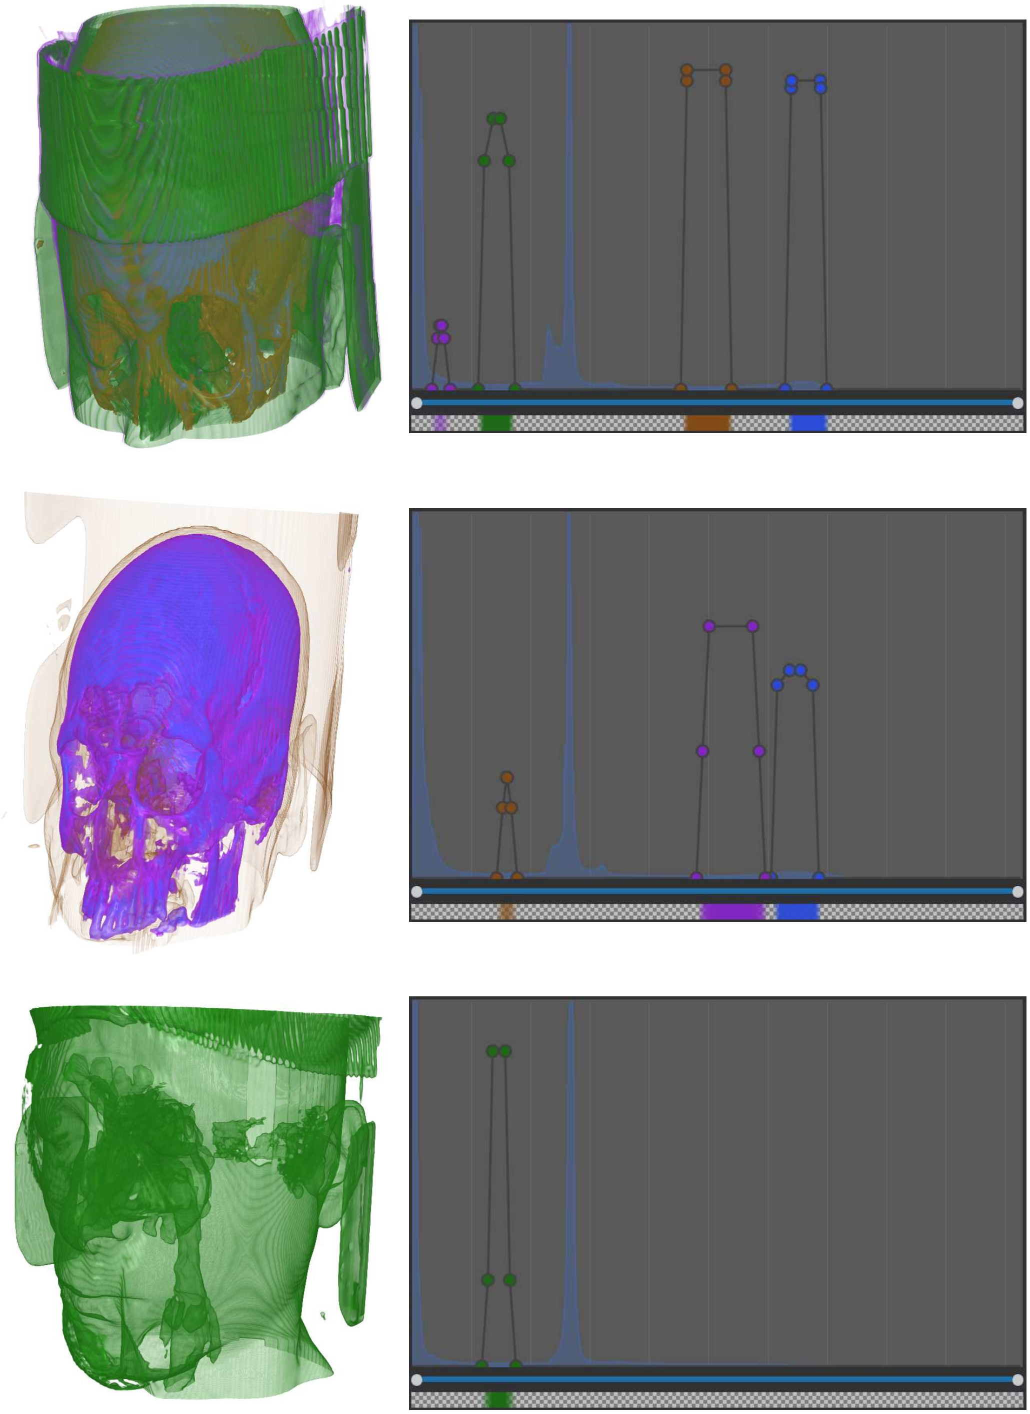

Figure 2: Examples of the data used for training DVAO. On the left is the input volume ($128^3$) rendered with the generated random transfer function (right). The TFs are displayed in the TF editor widget of Inviwo. These widgets encode the opacity as y-coordinate of the points and show the volume histogram in the background. Underneath is the resulting TF texture. Note that only the opacity values are used in the network and the colors are only used to distinguish the peaks of TF in the rendering.

# 4 Effects of increasing the network size

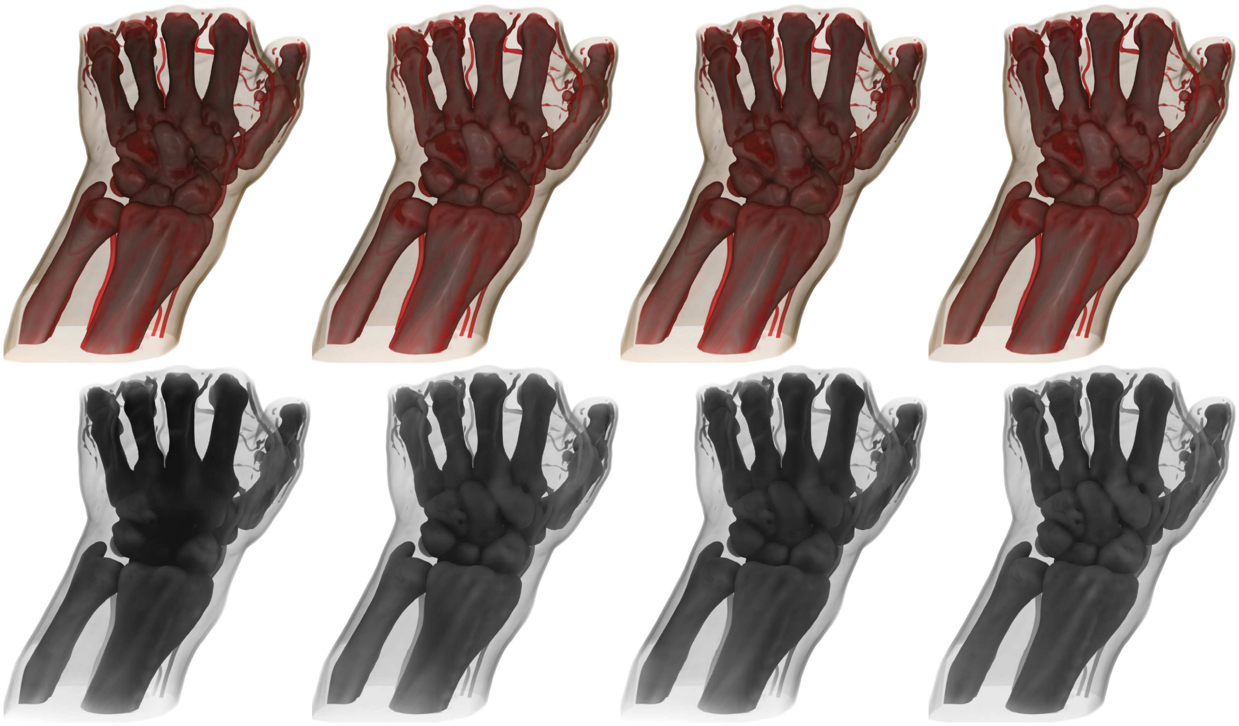

(a) No. Filters: 8 (b) No. Filters: 16 (c) No. Filters: 24 (d) Ground Truth

Figure 3: A comparison of rendered predictions (Full render top, AO only bottom) from models with different network sizes. We modify the *number of filters* in the first convolutional layer. This number of filters is doubled on every downsampling step in the CNN and thus controls the overall amount of parameters in the network. Our proposed default for this parameter is 16. We can see that halving the number of filters to 8 results in significantly less detailed AO volumes, while further increasing it to 24 does not improve the results.

# 5 Generalization to non-human CT data

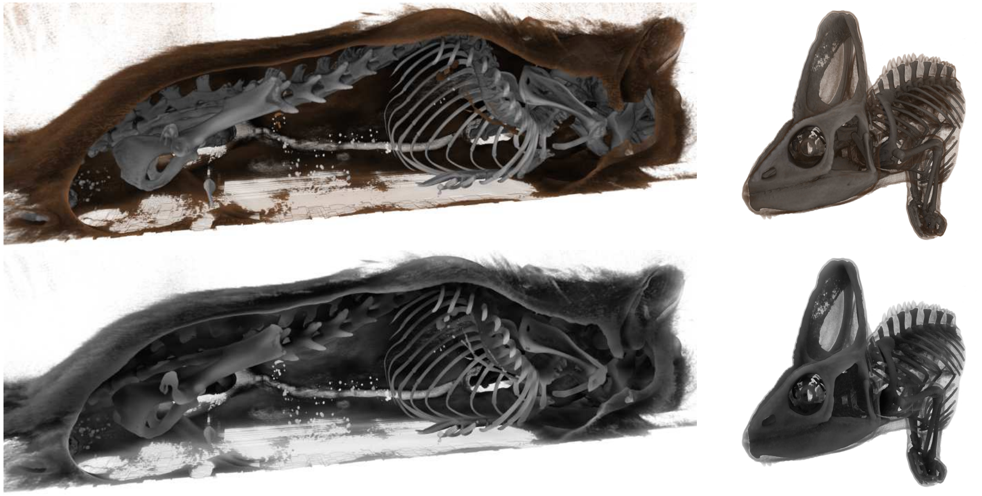

(a) Mouse Micro-CT
SSIM: 0.786, MSE: 0.024

(b) Chameleon CT
SSIM: 0.866, MSE: 0.026

Figure 4: Renders of non-human computed tomography data. Our neural network was only trained on scans of human heads. Those renders demonstrate that our approach can generalize beyond the head scans and performs well on CT scans of animals. Metrics are reported against ground truth.
